# Supplementary material for: Gating is Weighting: Understanding Gated Linear Attention through In-context Learning
Source: arXiv:2504.04308 source file (2025-04-06)
Supplement: Supplementary file 1 [file add_exp.tex]

\section{Experiments}
\begin{figure}[!t]
\centering
\begin{subfigure}{0.45\linewidth}    
\centering
\includegraphics[height=0.7\linewidth]{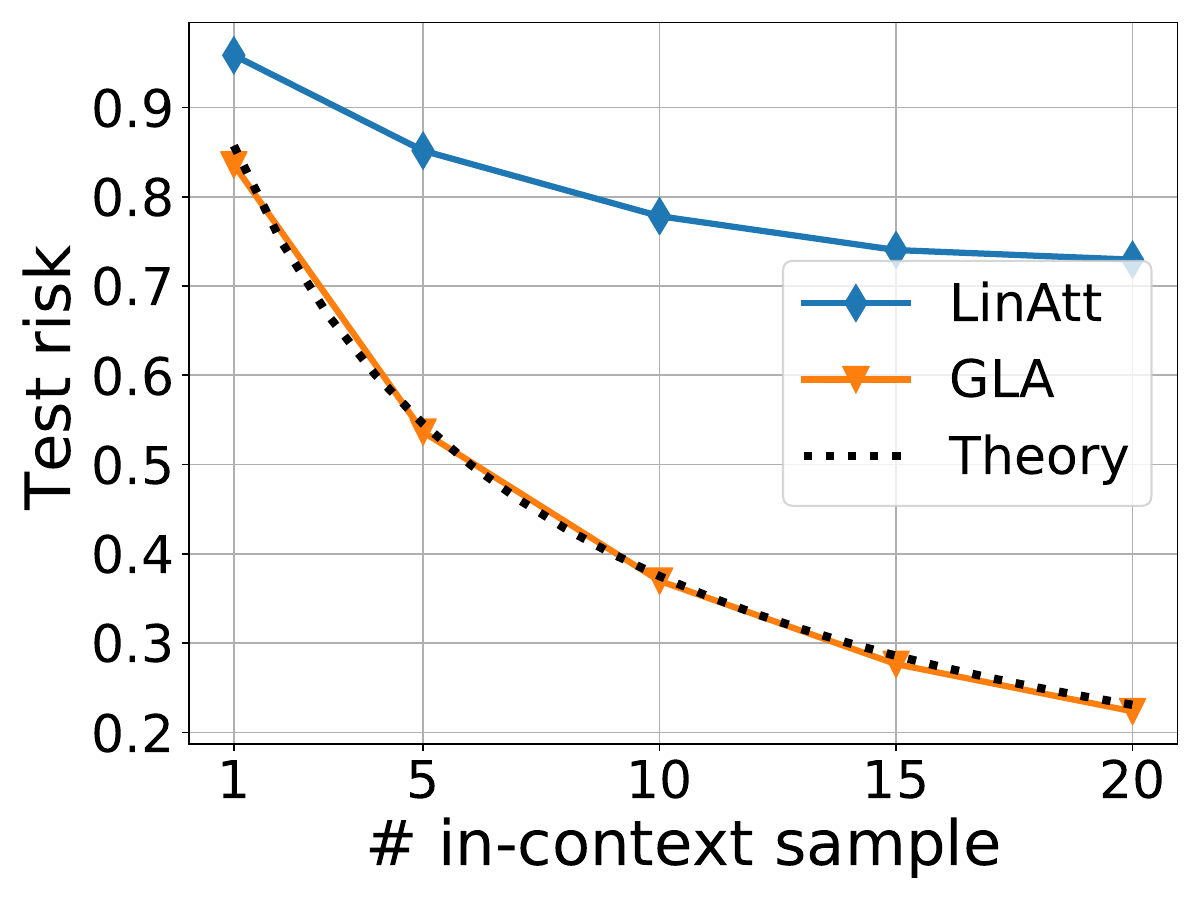}
\caption{Test risk}\label{fig:loss}
\end{subfigure}
\hspace{20pt}
\begin{subfigure}{0.45\linewidth}    
    \centering
    \includegraphics[height=.7\columnwidth]{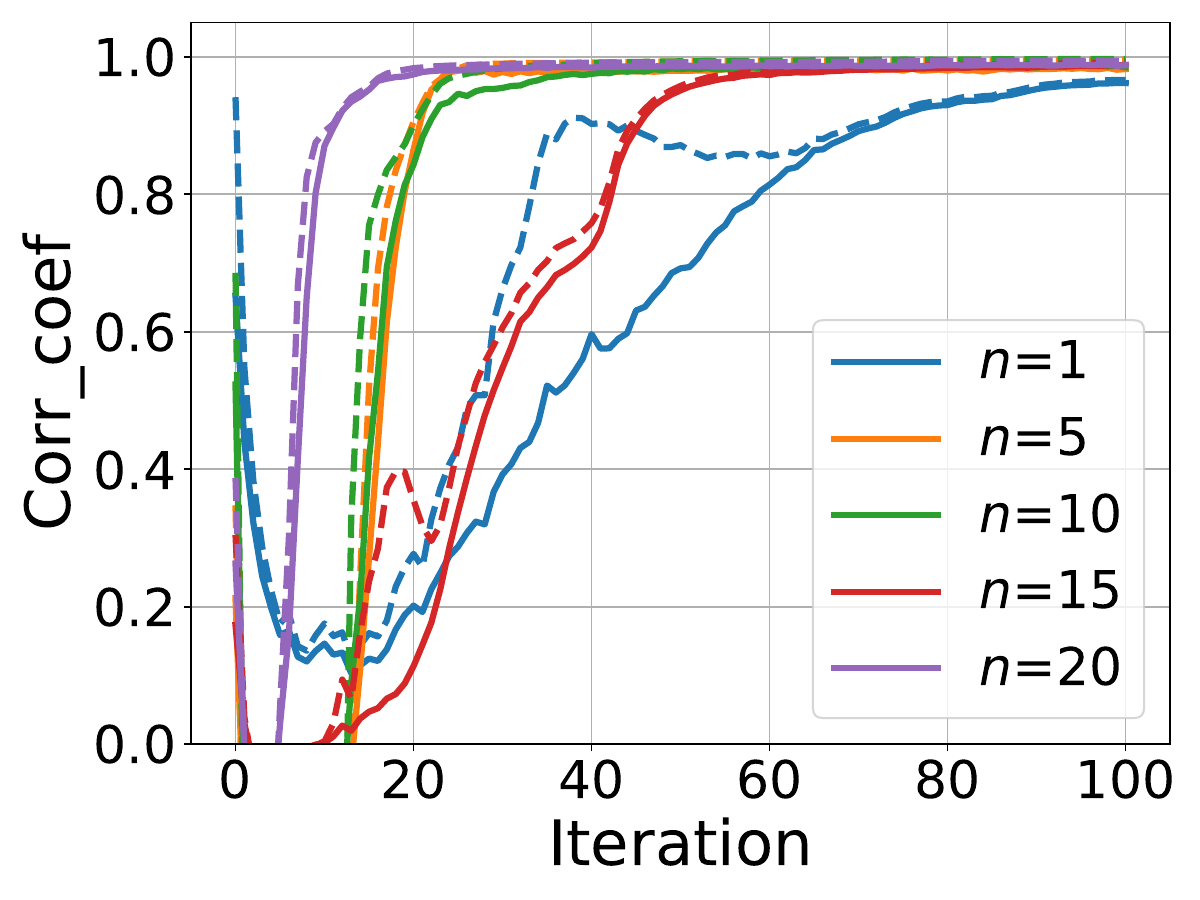}
\caption{Correlation coefficient}\label{fig:corr}
\end{subfigure}
\caption{\textbf{(a)} Train linear attention and GLA models with task-mixture prompts and evaluation results are presented in blue and orange curves, respectively. Here, theory curve (black dotted) is obtained via the Theorem~1 in \cite{li2024fine}. \textbf{(b)} Evolution of correlation coefficients of trained gating parameter $\hat\w_g$ with max-margin solutions obtained in \eqref{w mm}. Here, solid curves represent the results of corr\_coef($\hat\w_g,(\w')^{mm}_g$) where $(\w')^{mm}_g$ is an extended version of $\w^{mm}_g$ following \eqref{w mm extend}. Dashed curves display the results of corr\_coef($\hat\w_g[-d':],\w^{mm}_g$) where $\hat\w_g[-d':]$ returns the last $d'$ dimension of $\hat\w_g$.}\label{fig:iid k3}
\end{figure}

\begin{table}[]
    \centering
    \begin{tabular}{c|ccccc}
    \midrule
        $n$ & $1$ & $5$ & $10$ & $15$ & $20$ \\
    \midrule
        corr\_coef($\hat\w_g,(\w')^{mm}_g$) & $0.962$ & $0.982$ & $0.985$ & $0.988$ & $0.988$\\
    \midrule
        corr\_coef($\hat\w_g[-d':],\w^{mm}_g$) & $0.966$ & $0.996$ & $0.997$ & $0.992$ & $0.994$\\
    \midrule
    \end{tabular}
    \caption{Correlation coefficients of gating parameters with max-margin solutions.}
    \label{tab:iid k3}
\end{table}

\noindent\textbf{Data generation. } Consider task-mixture linear-ICL problem with dimension $d$. Suppose each input sequence contains $K$ tasks corresponding to task vectors $(\bt_k)_{k=1}^K$ where tasks follow the same distribution $\Dc_\bt$. In the experiments, let us assume $(\bt_k)_{k=1}^K\sim\Nc(0,\Iden)$. Then given context length (of each task) $n$, the prompt is constructed via
\[
\Z^\top =\begin{bmatrix}
    \X_1^\top&\zerobb&\X_2^\top&\zerobb&\cdots&\X_K^\top&\x\\
    \y_1^\top&0&\y_2^\top&0&\cdots&\y_K^\top&0\\
    \cb\onebb^\top&\db_1&\cb\onebb^\top&\db_2&\cdots&\cb\onebb^\top&\cb
\end{bmatrix}\in\R^{(d+1+d')\times K(n+1)}.
\]
Here $(\X_k,\y_k)\subset\R^{n\times d}\times\R^{n}=(\x_{ki},y_{ki})_{i=1}^n$ corresponds to task $\bt_k$ and is generated via $y_{ki}=\bt_k^\top\x_{ki}$. The delimiters are sampled from $\cb\in\Cb\subset\R^{d'}$ and $\db_{1,\cdots, K}\in\Db\subset\R^{d'}$. Note that to distinguish different tasks, within each prompt, $\db_{k}\neq\db_{k+1},k\in[K-2]$. Then, given prompt $\Z$ with query input $\x$, the goal is to predict $y=\x^\top\bt_K$.

\smallskip

\noindent\textbf{Experimental setting.} 
\begin{itemize}
    \item Choose $d=5,K=3$ and $d'=5$.
    \item All $\x_{ki}$, $\x$, and $\bt_k$ are sampled from $\Nc(0,\Iden_d)$.
    \item $|\Cb|=1$, $|\Eb|=K=3$ and elements are randomly sampled from $\Nc(0,\Iden_{d'})$.
    \item $\db_1\neq\db_2\neq\db_3$. Therefore, in the experiments, assume that $\{\db_1,\db_2,\db_3\}=\Eb$.
    \item \textbf{Gating function:} Consider gating function 
    \[
    g(\z_i)=\sigma(\w_g^\top\z_i)\onebb\onebb^\top\quad\text{where}\quad\w_g\in\R^{d+d'+1}~\text{and}~\sigma(z)=\frac{1}{1+e^{-z}}.
    \]
\end{itemize}

\noindent\textbf{Analysis.} Since different tasks $(\bt_{k})_{k=1}^K$ are uncorrelated, the optimal gating would be $[\zerobb^\top_{(K-1)(n+1)}~~\onebb^\top_{n}~~0]$ such that the prediction of $\Z$ with query $\x$ depended on the tokens sampled from $\bt_K$ only. We first show that the optimal gating vector is achievable given delimiters $\Cb$ and $\Eb$. Define the max-margin solution as follows:
\begin{align}
    \w_g^{mm}= \arg\min_{\w}~\tn{\w}\quad s.t.\quad \begin{cases}
        \w^\top\cb\geq1&\forall \cb\in\Cb\\
        \w^\top\db\leq-1&\forall \db\in\Db
    \end{cases}.\label{w mm}
\end{align}
Additionally, let 
\begin{align}
(\w')_g^{mm}=\begin{bmatrix}
    \zerobb_{d+1}\\
    \w_g^{mm}
\end{bmatrix}.\label{w mm extend}
\end{align}
Then $R\cdot(\w')_g^{mm}$ with $R\to\infty$ results in gating vector $[\zerobb^\top_{(K-1)(n+1)}~~\onebb^\top_{n}~~0]$, and following \cite{li2024fine}, the optimal normalized test risks are
\[
\Lc^\st_{gla}=1-\frac{1}{d+n+1}.
\]

\noindent\textbf{Experimental results. } Following the experimental setting discussed above, we repeat $10$ individual model trainings with different initialization, training data and $\Cb,\Db$ matrices. The results corresponding to the trail with minimal test risks are reported. We train the model with SGD optimizer and learning rate $\eta=0.001$. To ensure divergence of gating weights, we apply normalized gradient descent to it and therefore, $\w_g$ is updated via
\[
\w_g(t+1)=\w_g(t)-\eta\frac{\nabla_{\w_g(t)}\Lc_{gla}}{\tn{\nabla_{\w_g(t)}\Lc_{gla}}+10^{-20}}.
\]
Results are presented in Figure~\ref{fig:iid k3} and Table~\ref{tab:iid k3}.
