# Supplementary material for: Gating is Weighting: Understanding Gated Linear Attention through In-context Learning
Source: arXiv:2504.04308 source file (2025-04-06)
Supplement: Supplementary file 4 [file supp_wpgd.tex]

\section{Optimization Landscape of WPGD}
\label{sec:app:wpgd}
Recapping the objective from \eqref{eqn:wpgd:risk} and following Definition~\ref{def:multitask}, we can derive
\begin{align}
\Lc(\Pb,\bom)&=\E\left[\left(y-\x^\top \Pb \X(\bom \odot \y)\right)^2\right]\nn\\
&=\E\left[y^2\right]-2\E\left[y\x^\top\Pb\X(\bom\odot\y)\right]+\E\left[\left(\x^\top\Pb\X(\bom\odot\y)\right)^2\right].\nn%\\
% &=\tr{\bSi}+\sigma^2-2\E\left[\bt^\top\x\x^\top\Pb\sum_{i=1}^n\omega_i\x_i\x_i^\top\bt_i\right]+\E\left[\x\x^\top\Pb\left(\sum_{i=1}^n\omega_i\x_i\x_i^\top\bt_i\right)\left(\sum_{i=1}^n\omega_i\x_i\x_i^\top\bt_i\right)^\top\Pb^\top\right]\nn\\
% &=\tr{\bSi}+\sigma^2
\end{align}
Let $y=\x^\top\bt+\xi$ and $y_i=\x_i^\top\bt_i+\xi_i$, $i\in[n]$ where $\xi,\xi_i\sim\Nc(0,\sigma^2)$ are iid. Then
\[
\E[y^2]=\E[(\x^\top\bt+\xi)^2]=\tr{\bSi}+\sigma^2
\]
and
\begin{align*}
    \E\left[y\x^\top\Pb\X(\bom\odot\y)\right]&=\E\left[(\bt^\top\x+\xi)\x^\top\Pb\sum_{i=1}^n\omega_i\x_i(\x_i^\top\bt_i+\xi_i)\right]\\
    &=\E\left[\bt^\top\x\x^\top\Pb\sum_{i=1}^n\omega_i\x_i\x_i^\top\bt_i\right]\\
    &=\tr{\bSi\Pb\bSi\sum_{i=1}^n\omega_i\E\left[\bt_i\bt^\top\right]}\\
    &=\tr{\bSi^2\Pb}\bom^\top\rb.
\end{align*}
Here the last equality comes from the fact that since $\bt_i-r_{ij}\bt_j$ is independent of $\bt_j$ for $i,j\in[n+1]$ following Definition~\ref{corr task def}, we have $\E\left[\bt_i\bt^\top\right]=r_{i,n+1}\Iden_d$ and $\sum_{i=1}^n\omega_i\E\left[\bt_i\bt^\top\right]$ returns $\bom^\top\rb\cdot\Iden_d$. 
\begin{align*}
    \E\left[\left(\x^\top\Pb\X(\bom\odot\y)\right)^2\right]&=\E\left[\x^\top\Pb\left(\sum_{i=1}^n\omega_i(\x_i^\top\bt_i+\xi_i)\x_i\right)\left(\sum_{i=1}^n\omega_i\x_i^\top(\x_i^\top\bt_i+\xi_i)\right)\Pb^\top\x\right]\\
    &=\tr{\Pb^\top\bSi\Pb\E\left[\sum_{i=1}^n\omega_i^2(\x_i^\top\bt_i+\xi_i)^2\x_i\x_i^\top+\sum_{i\neq j}\omega_i\omega_j(\x_i^\top\bt_i+\xi_i)\x_i\x_j^\top(\x_j^\top\bt_j+\xi_j)\right]}%\\
    % &=\tr{\Pb^\top\bSi\Pb\E\left[\sum_{i=1}^n\omega_i^2(\x_i^\top\bt_i+\xi_i)^2\x_i\x_i^\top+\sum_{i\neq j}\omega_i\omega_j(\x_i^\top\bt_i+\xi_i)\x_i\x_j^\top(\x_j^\top\bt_j+\xi_j)\right]}
\end{align*}
where
\begin{align*}
    \tr{\Pb^\top\bSi\Pb\E\left[\sum_{i=1}^n\omega_i^2(\x_i^\top\bt_i+\xi_i)^2\x_i\x_i^\top\right]}&=\tr{\Pb^\top\bSi\Pb\E\left[\sum_{i=1}^n\omega_i^2(\x_i^\top\bt_i\bt_i^\top\x_i+\sigma^2)\x_i\x_i^\top\right]}\\
    &=\tn{\bom}^2\tr{\Pb^\top\bSi\Pb\left(\E\left[\x\x^\top\x\x^\top\right]+\sigma^2\bSi\right)}\\
    &=\tn{\bom}^2\left(\tr{\bSi\Pb^\top\bSi\Pb}\left(\tr{\bSi}+\sigma^2\right)+\tr{\bSi^2\Pb^\top\bSi\Pb}\right)
\end{align*}
and
\begin{align*}
    \tr{\Pb^\top\bSi\Pb\E\left[\sum_{i\neq j}\omega_i\omega_j(\x_i^\top\bt_i+\xi_i)\x_i\x_j^\top(\x_j^\top\bt_j+\xi_j)\right]}&=\tr{\Pb^\top\bSi\Pb\E\left[\sum_{i\neq j}\omega_i\omega_j\x_i\x_i^\top\bt_i\bt_j^\top\x_j\x_j^\top\right]}\\
    &=\tr{\bSi^2\Pb^\top\bSi\Pb}\bom^\top\Rb\bom.
\end{align*}
Combining all together and letting $M:=\tr{\bSi}+\sigma^2$, we obtain
{\color{red}
\begin{align}
    \Lc(\Pb,\bom)=M-2\tr{\bSi^2\Pb}\bom^\top\rb+M\tn{\bom}^2\tr{\bSi\Pb^\top\bSi\Pb}+(\tn{\bom}^2+\bom^\top\Rb\bom)\tr{\bSi^2\Pb^\top\bSi\Pb}.\label{app:loss}
\end{align}
}
% \begin{align*}
% \Lc(\Pb,\bom) &=-2\bom^\top \rb\cdot\tr{\bSi\Pb}+\bom^\top \Rb\bom \cdot\tr{\bSi^2\Pb^2}
% +\tn{\bom}^2\cdot \left(\tr{\bSi}\tr{\bSi\Pb^2}+\tr{\bSi^2\Pb^2}\right) +M .
% \end{align*}
Then differentiating with respect to $\Pb$ and $\bom$ returns
{\color{red}
\begin{align}
&\nabla_\Pb\Lc(\Pb,\bom)=-2\bom^\top\rb\bSi^2+2M\tn{\bom}^2\bSi^2\Pb+2(\tn{\bom}^2+\bom^\top\Rb\bom)\bSi^3\Pb\label{app:gd P}\\
&\nabla_{\bom}\Lc(\Pb,\bom)=-2\tr{\bSi^2\Pb}\rb+2M\tr{\bSi\Pb^\top\bSi\Pb}\bom+2\tr{\bSi^2\Pb^\top\bSi\Pb}(\Iden_n+\Rb)\bom.\label{app:gd w}
\end{align}
}

\subsection{Supporting Results}
\begin{lemma}\label{lem:quadL}
Let 
\begin{align}\label{eqn:gamma}
 \gamma := \frac{\bom^\top\Rb\bom}{\tn{\bom}^2} +1.   
\end{align}
The objective $\Lc(\Pb,\bom)$ in \eqref{eqn:wpgd:risk} has the following form 
\begin{align*}
\Lc(\Pb,\bom)=\left(\tr{\bSi}\tr{\bSi\Pb^2}+\gamma\tr{\bSi^2\Pb^2}\right) \cdot \tn{\bom}^2 -2\tr{\bSi\Pb} \cdot \bom^\top \rb+d.   
\end{align*}
%and is convex in both $\bom$ and $\Pb$.
\end{lemma}
\begin{proof}
Expanding $\X^\top (\bom \odot \y) = \sum_{i=1}^n w_i \x_i \x_i^\top \bt_i$ and using the symmetry of $\Pb$, we find that
\begin{subequations}\label{eqn:wpgd:obj1}
\begin{equation}
\begin{split}
\Lc(\Pb,\bom)-d&=\E[\sum_{i,j=1}^n w_iw_j\bt_i^\top\x_i\x_i^\top\Pb^2\x_j\x_j^\top\bt_j]-2\cdot\E[\sum_{i=1}^n w_i\bt^\top\Pb\x_i\x_i^\top\bt_i]\\
&=-2\bom^\top \rb\cdot\tr{\bSi\Pb}+\bom^\top \Rb\bom \cdot\tr{\bSi^2\Pb^2}+\texttt{rest},
\end{split}    
\end{equation}
where
\begin{equation}
\begin{split}
\texttt{rest} &:=\sum_{i=1}^n \omega_i^2 \left(\E[\tr{\x_i\x_i^\top\Pb^2\x_i\x_i^\top}]-\tr{\Pb^2\bSi^2}\right)\\
&= \tn{\bom}^2 \left(\E[\tn{\x}^2\x^\top\Pb^2\x]-\tr{\bSi^2\Pb^2}\right).    
\end{split}       
\end{equation}

\end{subequations}

Note that both \( \Pb \) and \( \bSi \) are symmetric matrices. Let \( \tilde{\W} = \sqrt{\bSi} \Pb^2 \sqrt{\bSi} \) and \( \W = \bSi \). Utilizing the whitening transformation \( \x = \sqrt{\bSi} \ub \), where \( \ub \sim \mathcal{N}(0, \mathbf{I}_d) \), we observe:
%Let $\ub\sim\Nc(0,\Iden_d)$. Then, for any $\W,\tilde{\W}\in\R^{d\times d}$, we have
\begin{align}\label{eqn:moment}
\nonumber
      \E\left[(\ub^\top\W\ub)(\ub^\top\tilde{\W}\ub)\right]
%&=\E\left[\left(\sum_{i,j=1}^dW_{ij}u_iu_j\right)\left(\sum_{i,j=1}^dW'_{ij}u_iu_j\right)\right]\nn\\
%&=\E\left[\left(\sum_{i=1}^dW_{ii}u_i^2\right)\left(\sum_{i=1}^dW'_{ii}u_i^2\right)\right]+\E\left[\left(\sum_{i\neq j}W_{ij}u_iu_j\right)\left(\sum_{i\neq j}W_{ij}'u_iu_j\right)\right]\nn\\
&=\sum_{i=1}^dw_{ii}\tilde{w}_{ii}\E\left[u_i^4\right]+\sum_{i\neq j}w_{ii}\tilde{w}_{jj}\E[u_i^2]\E[u_j^2]\\
\nonumber
&+\sum_{i\neq j}w_{ij}\tilde{w}_{ij}\E[u_i^2]\E[u_j^2]+\sum_{i\neq j}w_{ij}\tilde{w}_{ji}\E[u_i^2]\E[u_j^2]\nn\\
% &=3\sum_{i=1}^dW_{ii}\tilde{w}_{ii}+\sum_{i\neq j}W_{ii}\tilde{w}_{jj}+\sum_{i\neq j}W_{ij}\tilde{w}_{ij}+\sum_{i\neq j}W_{ij}\tilde{w}_{ji}\nn\\
% &=\sum_{i,j=1}^dW_{ii}\tilde{w}_{jj}+\sum_{i,j=1}^dW_{ij}\tilde{w}_{ij}+\sum_{i,j=1}^dW_{ij}W'_{ji}\nn\\
&=\tr{\W}\tr{\tilde{\W}}+\tr{\tilde{\W}\W^\top}+\tr{\W\tilde{\W}}.  
\end{align}
Hence, 
\begin{align*}
\E[\|\x\|^2 \x^\top \Pb^2 \x] %&= \tr{\bSi} \tr{\bSi \Pb^2} + \E \left[ \sum_{i=1}^d (\bar{x}_i^4 - 1) \bSi_{i,i} (\sqrt{\bSi} \Pb^2 \sqrt{\bSi})_{i,i} \right] \\
&= \tr{\bSi} \tr{\bSi \Pb^2} + 2 \tr{\bSi^2 \Pb^2}.
\end{align*}
Substituting the above equality in \eqref{eqn:wpgd:obj1} gives
\begin{equation}\label{eqn:wpgd:obj2}
    \begin{split}
\Lc(\bom)-d &=-2\bom^\top \rb\cdot\tr{\bSi\Pb}+\bom^\top \Rb\bom \cdot\tr{\bSi^2\Pb^2}\\
&+\tn{\bom}^2\cdot \left(\tr{\bSi}\tr{\bSi\Pb^2}+\tr{\bSi^2\Pb^2}\right).       
    \end{split}
\end{equation}
Recall from the statement of Lemma~\ref{lem:quadL} that 
\begin{align*}
\gamma = \frac{\bom^\top\Rb\bom}{\tn{\bom}^2} +1.
\end{align*}
It follows from \eqref{eqn:wpgd:obj2} that  
\begin{align*}
\Lc(\Pb,\bom)-d &=-2\bom^\top \rb\cdot\tr{\bSi\Pb}+\tn{\bom}^2\cdot \left(\tr{\bSi}\tr{\bSi\Pb^2}+\gamma\tr{\bSi^2\Pb^2}\right).    
\end{align*}
This completes the proof of the lemma.
\end{proof}

\subsection{Proof of  Theorem~\ref{thm:unique:wpgd} }
\begin{proof}
Recall the definition of $\gamma$ and the reformulation of $\Lc(\Pb, \bom)$ in Lemma~\ref{lem:quadL}. Differentiating with respect to $\Pb$ and $\bom$, we have
\begin{subequations}
\begin{equation}
    \begin{split}
       \nabla_{\bom} \Lc(\Pb,\bom) &= -2\rb\cdot\tr{\bSi\Pb} + 2\Rb\bom \cdot\tr{\bSi^2\Pb^2} \\
 &+ 2\bom\cdot \left(\tr{\bSi}\tr{\bSi\Pb^2}+\tr{\bSi^2\Pb^2}\right),   
    \end{split}
\end{equation}
and 
\begin{equation}
  \nabla_{\Pb} \Lc(\Pb,\bom)=  2 \tn{\bom}^2\left(\tr{\bSi}\bSi + \gamma\bSi^2\right)\Pb - 2\bom^\top\rb \cdot \bSi.   
\end{equation}
\end{subequations}
By setting the above gradients equal to zero, we obtain
\begin{subequations}
\begin{equation}\label{eqn:p:opt1}
    \begin{split}
&\Pb = \frac{\bom^\top\rb}{\tn{\bom}^2\tr{\bSi}}\cdot \left( \frac{\gamma}{\tr{\bSi}}\cdot \bSi+\Iden \right)^{-1},
    \end{split}
\end{equation}
\begin{equation}\label{eqn:w:opt1}
    \begin{split}
&\bom= \frac{\tr{\bSi\Pb}}{ \tr{\bSi^2\Pb^2}+\tr{\bSi} \tr{\bSi\Pb^2}}\\
& \quad\cdot \left( \frac{\tr{\bSi^2\Pb^2}}{\tr{\bSi^2\Pb^2}+\tr{\bSi} \tr{\bSi\Pb^2}}\cdot\Rb+\Iden\right)^{-1}\rb.
    \end{split}
\end{equation}
\end{subequations}
% Given this, $\Pb$ admits the closed form solution 
% \begin{align*}
% &\Pb=\bom^\top\rb\cdot \left(\bom^\top(\Rb+\Iden)\bom\cdot \bSi^2+\tn{\bom}^2\tr{\bSi}\bSi\right)^{-1}\\
% &=\frac{\bom^\top\rb}{\tn{\bom}^2\tr{\bSi}}\cdot \left( \frac{\bom^\top\Rb\bom+\tn{\bom}^2}{\tn{\bom}^2\tr{\bSi} }\bSi^2+\bSi\right)^{-1}\\
% %&= C_{\bom}\left( \bgam \bSi^2+\bSi\right)^{-1}\\
% & = C_{\bom} \cdot \bSi^{-1}\left( \frac{\gamma+1}{\tr{\bSi}} \bSi+\Iden\right)^{-1}\\
% & = C_{\bom} \cdot \bSi^{-1} \bSi_{\gamma}^{-1}.  
% \end{align*}
% where 
% \begin{align}
%     C_{\bom} := \frac{\bom^\top\rb}{\tn{\bom}^2\tr{\bSi}}. 
% \end{align}
Let 
\begin{align}
 \bSi_{\gamma} := \frac{\gamma}{\tr{\bSi}} \bSi + \Iden.  
\end{align}

\begin{align*}
    \abs{\frac{\partial g}{\partial \gamma}}&\leq \frac{\left(\sum_{i=1}^d \frac{s_i^3}{\left(M+\gamma s_i\right)^2}\right)^2}{\left(M\sum_{i=1}^d \frac{s_i^2}{\left(M+\gamma s_i\right)^2}\right)^2}\cdot M^2 \cdot\left(\sum_{i=1}^d \frac{s_i^3}{\left(M+\gamma s_i\right)^2}\right)^{-2}\sum_{i,j=1}^d \frac{s_i^2 s_j^2 (s_i-s_j)^2}{\left(M+\gamma s_i\right)^3\left(M+\gamma s_j\right)^3}\\
    &=\left(\sum_{i=1}^d \frac{s_i}{\left(M+\gamma s_i\right)^2}\right)^{-2}\sum_{i,j=1}^d \frac{s_i^2s_j^2(s_i-s_j)^2}{\left(M+\gamma s_i\right)^3\left(M+\gamma s_j\right)^3}<1
\end{align*}

\begin{align*}
    \abs{\frac{\partial g}{\partial \gamma}}&\leq \frac{\left(\sum_{i=1}^d \frac{s_i^3}{\left(M+\gamma s_i\right)^2}\right)^2}{\left(M\sum_{i=1}^d \frac{s_i^2}{\left(M+\gamma s_i\right)^2}\right)^2}\cdot M^2 \cdot\left(\sum_{i=1}^d \frac{s_i^3}{\left(M+\gamma s_i\right)^2}\right)^{-2}\sum_{i,j=1}^d \frac{s_i^2 s_j^2 (s_i-s_j)^2}{\left(M+\gamma s_i\right)^3\left(M+\gamma s_j\right)^3}\\
    &=\left(\sum_{i=1}^d \frac{s_i}{\left(M+\gamma s_i\right)^2}\right)^{-2}\sum_{i,j=1}^d \frac{s_i^2s_j^2(s_i-s_j)^2}{\left(M+\gamma s_i\right)^3\left(M+\gamma s_j\right)^3}<1
\end{align*}

Let 
\begin{align}
 \bSi_{\gamma} := \frac{\gamma}{\tr{\bSi}} \bSi + \Iden.  
\end{align}
Let the scalar function $g: \mathbb{R}_{+} \rightarrow \mathbb{R}_{+}$ be defined by
\begin{equation}\label{func:g(gamma)}
    \begin{split}
 g(\gamma) &: = \left(1+ 
\tr{\bSi} \frac{\tr{\bSi \bSi^{-2}_{\gamma}}}{\tr{\bSi^2  \bSi^{-2}_{\gamma}} }\right)^{-1}\\
%& =  \frac{\sum_{i=1}^n \frac{s_i^2}{(1+\gamma s_i)^2}}{\sum_{i=1}^n \frac{s_i^2}{(1+\gamma s_i)^2}+ (\sum_{i=1}^n s_i)\sum_{i=1}^n \frac{s_i}{(1+\gamma s_i)^2}},  
&= \left( 1+ \tr{\bSi} \left(\sum_{i=1}^d \frac{s_i^2}{\left(\tr{\bSi}+\gamma s_i\right)^2}\right)^{-1} \sum_{i=1}^d \frac{s_i}{\left(\tr{\bSi}+\gamma s_i\right)^2}\right)^{-1}.\\
\frac{\partial g}{\partial \gamma}&=-g(\gamma)^2\tr{\bSi}^2\left(\sum_{i=1}^d \frac{s_i^2}{\left(\tr{\bSi}+\gamma s_i\right)^2}\right)^{-2}\sum_{i,j=1}^d \frac{s_is_j(s_i-s_j)^2}{\left(\tr{\bSi}+\gamma s_i\right)^3\left(\tr{\bSi}+\gamma s_j\right)^3}
    \end{split}
\end{equation}

\begin{align*}
    \abs{\frac{\partial g}{\partial \gamma}}&\leq\frac{\left(\sum_{i=1}^d \frac{s_i^2}{\left(\tr{\bSi}+\gamma s_i\right)^2}\right)^2}{\left(\tr{\bSi}\sum_{i=1}^d \frac{s_i}{\left(\tr{\bSi}+\gamma s_i\right)^2}\right)^2}\cdot\tr{\bSi}^2\cdot\left(\sum_{i=1}^d \frac{s_i^2}{\left(\tr{\bSi}+\gamma s_i\right)^2}\right)^{-2}\sum_{i,j=1}^d \frac{s_is_j(s_i-s_j)^2}{\left(\tr{\bSi}+\gamma s_i\right)^3\left(\tr{\bSi}+\gamma s_j\right)^3}\\
    &=\left(\sum_{i=1}^d \frac{s_i}{\left(\tr{\bSi}+\gamma s_i\right)^2}\right)^{-2}\sum_{i,j=1}^d \frac{s_is_j(s_i-s_j)^2}{\left(\tr{\bSi}+\gamma s_i\right)^3\left(\tr{\bSi}+\gamma s_j\right)^3}<1
\end{align*}

Here, the equality follows from  eigen decomposition $\bSi=\Ub \textnormal{diag}(\mathbf{s})\Ub^\top$ with  $\s = [s_1, \ldots, s_d]^\top \in \R^d_{+}$.

Now, plugging $\Pb$ defined in \eqref{eqn:p:opt1} within $\bom$ given in \eqref{eqn:w:opt1}, we obtain
\red{\begin{align}\label{eqn:w:opt2}
\bom = \frac{  \tn{\bom}^2 \tr{\bSi} \tr{\bSi \bSi^{-1}_{\gamma}}}{  \bom^\top\rb  \left( \tr{\bSi  \bSi^{-2}_{\gamma}} + \tr{\bSi} \tr{\bSi  \bSi^{-2}_{\gamma}} \right)} \cdot\left(g(\gamma) \cdot \Rb+\Iden\right)^{-1}\rb.
\end{align}}
Using the above formulae for $\bom$, we rewrite $\gamma$ in \eqref{eqn:gamma} as
\begin{equation}\label{eqn:comps1}
\begin{split}
    \gamma &= \frac{\rb^\top (  g(\gamma) \Rb+\Iden)^{-1}\Rb(  g(\gamma) \Rb+\Iden)^{-1}\rb}{ \rb^\top (  g(\gamma) \Rb+\Iden)^{-2}\rb} +1\\
%&= \frac{\sum_{i=1}^n \frac{\la_ia_i^2}{(1+  g(\gamma) \la_i)^2}}{\sum_{i=1}^n \frac{a_i^2}{(1+g(\gamma)  \la_i)^2}}\\
%&=\left( 1+ \sum_{i=1}^d s_i \left(\sum_{i=1}^d \frac{s_i^2}{\left(1+\gamma s_i\right)^2}\right)^{-1} \sum_{i=1}^d \frac{s_i}{\left(1+\gamma s_i\right)^2}\right)^{-1}\\
&= \sum_{i=1}^n \frac{\la_ia_i^2}{ \left(1+  g(\gamma) \la_i\right)^2} \left(\sum_{i=1}^n \frac{a_i^2}{\left(1+g(\gamma)  \la_i\right)^2}\right)^{-1}+1\\
&=: h\left(g\left(\gamma\right)\right),  
\end{split}    
\end{equation}
where the second equality follows since $\Rb = \Eb \text{diag}(\bla) \Eb^\top$ denotes the eigen decomposition of $\Rb$, where $\s = [s_1, \ldots, s_d]^\top \in \R^d_{+}$ and $\bla = [\lambda_1, \ldots, \lambda_n]^\top \in \R^n_{+}$, and by our assumption $\rb = \Eb \ab$ for some $\ab = [a_1, \ldots, a_n]^\top \in \R^n_{+}$.

\end{proof}

\subsection{Backup: Generic R}

\begin{lemma}
Let the functions \( h: \mathbb{R}_{+} \to \mathbb{R}_{+} \) and \( g: \mathbb{R}_{+}  \to  \mathbb{R}_{+} \) be defined as
\begin{align}
      h(\bar{\gamma}) &= \sum_{i=1}^n \frac{\lambda_i a_i^2}{ \left(1+\bar{\gamma} \lambda_i\right)^2} \left(\sum_{i=1}^n \frac{a_i^2}{\left(1+ \bar{\gamma}  \lambda_i\right)^2}\right)^{-1}, \\
      g(\gamma) &=  \left(1 + \left( \sum_{i=1}^d s_i \right) 
\left( \sum_{i=1}^d \frac{s_i^2}{\left( \sum_{i=1}^d s_i + (\gamma+1) s_i \right)^2} \right)^{-1}
\sum_{i=1}^d \frac{s_i}{\left( \sum_{i=1}^d s_i + (\gamma+1) s_i \right)^2}\right)^{-1}.
\end{align}
We claim that \( | h'(g(\gamma)) \cdot  g'(\gamma) | < 1 \).
\end{lemma}

\begin{proof}
Let
\begin{align*}
A(g) &:= \sum_{i=1}^n \frac{\lambda_i a_i^2}{(1+g\lambda_i)^2}, \qquad A'(g) := -2 \sum_{i=1}^n \frac{\lambda_i^2 a_i^2}{(1+g\lambda_i)^3}, \\
B(g) &:= \sum_{i=1}^n \frac{a_i^2}{(1+g\lambda_i)^2}, \qquad B'(g) := -2 \sum_{i=1}^n \frac{\lambda_i a_i^2}{(1+g\lambda_i)^3}.
\end{align*}
The derivative of $h$ with respect to \( g \) is given by
\begin{align*}
     \frac{\partial h}{\partial g} = \frac{B(g)A'(g) - A(g)B'(g)}{B(g)^2}.
\end{align*}
We begin by bounding each term in \( \frac{\partial h}{\partial g} \). First, observe that
\begin{align*}
%\label{eq:bounds_BA}
- \frac{\lambda_{\max}^2}{(1 + g \lambda_{\min})} \left(\sum_{i=1}^n \frac{a_i^2}{(1 + g \lambda_i)^2}\right)^{2}  &\leq B(g) A'(g) \leq  -\frac{\lambda_{\min}^2}{(1 + g \lambda_{\max})} \left(\sum_{i=1}^n \frac{a_i^2}{(1 + g \lambda_i)^2}\right)^{2}, \\
\frac{\lambda_{\min}^2}{(1 + g \lambda_{\max})} \left(\sum_{i=1}^n \frac{a_i^2}{(1 + g \lambda_i)^2}\right)^{2} &\leq A(g) B'(g) \leq \frac{\lambda_{\max}^2}{(1 + g \lambda_{\min})} \left(\sum_{i=1}^n \frac{a_i^2}{(1 + g \lambda_i)^2}\right)^{2}.
\end{align*}
Using the above bounds, we deduce that
\begin{align*}
-\frac{\lambda_{\max}^2}{(1 + g \lambda_{\min})} + \frac{\lambda_{\min}^2}{(1 + g \lambda_{\max})} &\leq \frac{\partial h}{\partial g} \leq - \frac{\lambda_{\min}^2}{(1 + g \lambda_{\max})} + \frac{\lambda_{\max}^2}{(1 + g \lambda_{\min})}.
\end{align*}

Thus, the bounds on \( \frac{\partial h}{\partial g} \) give us
\begin{align*}
-\kappa^2 + \frac{1}{1 + \lambda_{\max}} \leq \frac{\partial h}{\partial g} \leq -\frac{1}{1 + \lambda_{\max}} + \kappa^2,
\end{align*}
where $\kappa=\lambda_{\max}/ \lambda_{\min}$.

Hence, we have
\begin{align}\label{eqn:partial:hg:bound}
    \left|\frac{\partial h}{\partial g}\right| \leq \kappa^2 - \frac{1}{1 + \lambda_{\max}}.
\end{align}

Let \( S = \sum_{i=1}^d s_i \) and \( D_i(\gamma) = S + (\gamma+1) s_i \).
We have
\[
B(\gamma) = \sum_{i=1}^d \frac{s_i^2}{D_i(\gamma)^2}, \quad C(\gamma) = \sum_{i=1}^d \frac{s_i}{D_i(\gamma)^2}, \quad A(\gamma) = 1 + S \frac{C(\gamma)}{B(\gamma)}.
\]

The derivatives of \( B(\gamma) \) and \( C(\gamma) \) are
\[
B'(\gamma) = -2 \sum_{i=1}^d \frac{s_i^3}{D_i(\gamma)^3}, \quad C'(\gamma) = -2 \sum_{i=1}^d \frac{s_i^2}{D_i(\gamma)^3}.
\]

Note that in the case $d=1$, we have $g(\gamma) =0$. Hence, we assume $d\geq2$. 
The gradient of \( g(\gamma) \) is
\begin{align*}
 g'(\gamma) &= - \frac{S }{A(\gamma)^2} \cdot \frac{C'(\gamma) B(\gamma) - C(\gamma) B'(\gamma)}{B(\gamma)^2} \\
 & =- \frac{S }{A(\gamma)^2 B(\gamma)^2} \cdot \left(C'(\gamma) B(\gamma) - C(\gamma) B'(\gamma)\right).
\end{align*}

We can bound the terms \( C'(\gamma)B(\gamma) \) and \( C(\gamma)B'(\gamma) \) as follows:
\begin{align*}
\left(\sum_{i=1}^d \frac{s_i^2}{D_i(\gamma)^2}\right)^2  \cdot   \frac{1}{S + (\gamma+1) s_{\max} } &\leq - C'(\gamma) B(\gamma) \leq  \left(\frac{ 1}{S + (\gamma+1) s_{\min} }\right)  \cdot \left(\sum_{i=1}^d \frac{s_i^2}{D_i(\gamma)^2}\right)^2, \\
 \left(\sum_{i=1}^d \frac{s_i^2}{D_i(\gamma)^2}\right)^2 \cdot \frac{-s_{\max}}{s_{\min}(S + (\gamma+1) s_{\min})}  &\leq  C(\gamma) B'(\gamma)  \leq  \frac{-s_{\min} }{s_{\max}(S + (\gamma+1) s_{\max})} \cdot \left(\sum_{i=1}^d \frac{s_i^2}{D_i(\gamma)^2}\right)^2.
\end{align*}
Thus, we obtain  
\begin{align*}
   \frac{1}{S + (\gamma+1) s_{\max} } &\leq - \frac{C'(\gamma) B(\gamma)}{B(\gamma)^2} \leq  \frac{ 1}{S + (\gamma+1) s_{\min} }, \\
\frac{-s_{\max}}{s_{\min}(S + (\gamma+1) s_{\min})}  &\leq \frac{ C(\gamma) B'(\gamma)}{B(\gamma)^2}  \leq  \frac{-s_{\min} }{s_{\max}(S + (\gamma+1) s_{\max})}.
\end{align*}

Next, we know that \( A(\gamma)^2 \geq 1 \), and we can bound \( \frac{1}{A^2(\gamma)} \) as
\[
\left(1+ S \frac{\sum_i \frac{s_i}{(S+(\gamma+1)s_i)^2}}{\sum_i \frac{s_i^2}{(S+(\gamma+1)s_i)^2}} \right)^{-2} \leq \frac{1}{A^2(\gamma)}\leq \left( 1+ S \frac{\sum_i \frac{s_i}{(S+(\gamma+1)s_i)^2}}{\sum_i \frac{s_i^2}{(S+(\gamma+1)s_i)^2}}\right)^{-2}.
\]
This simplifies to
\[
\left(1+ \frac{S}{s_{\min}}\right)^{-2} \leq \frac{1}{A^2(\gamma)}\leq \left( 1+ \frac{S}{s_{\max}}\right)^{-2}.
\]
Let \( \kappa_1 = \frac{s_{\max}}{s_{\min}} \), we have
\[
\left(1+ \kappa_1\right)^{-2} \leq \frac{1}{A^2(\gamma)} \leq \left( 1+ \frac{1}{\kappa_1}\right)^{-2}.
\]

Substituting these into the bounds for \( g'(\gamma) \), we get
\begin{align*}
\left(1+ \kappa_1\right)^{-2}  \cdot  \frac{1}{S + (\gamma+1) s_{\max} } &\leq - \frac{C'(\gamma) B(\gamma)}{A(\gamma)^2 B(\gamma)^2} \leq  \left(\frac{ 1}{S + (\gamma+1) s_{\min} }\right) \cdot \left( 1+ \frac{1}{\kappa_1}\right)^{-2}, \\
\left( 1+ \frac{1}{\kappa_1}\right)^{-2} \cdot \frac{-s_{\max}}{s_{\min}(S + (\gamma+1) s_{\min})}  &\leq \frac{ C(\gamma) B'(\gamma)}{A(\gamma)^2 B(\gamma)^2}  \leq  \frac{-s_{\min} }{s_{\max}(S + (\gamma+1) s_{\max})} \cdot \left(1+ \kappa_1\right)^{-2}.
\end{align*}

As \( \gamma \rightarrow 0 \), the bounds reduce to
\begin{align*}
\left(1+ \kappa_1\right)^{-3}  &\leq - \frac{ S \cdot C'(\gamma) B(\gamma)}{A(\gamma)^2 B(\gamma)^2} \leq \frac{\kappa_1^2}{(1+\kappa_1)^3}, \\
\frac{-\kappa_1^3}{(\kappa_1 + 1)^2 \left(1 + \frac{s_{\min}}{S}\right)}  &\leq \frac{ S \cdot C(\gamma) B'(\gamma)}{A(\gamma)^2 B(\gamma)^2}  \leq \frac{-1 }{\kappa_1\left(1+ \frac{s_{\max}}{S}\right)} \cdot \left(1+ \kappa_1\right)^{-2}.
\end{align*}

Thus, combining the results
\begin{align*}
    \left(1 + \kappa_1\right)^{-3} \left(1 - \frac{\kappa_1^3 \cdot (1 + \kappa_1)}{1 + d \kappa_1}\right) \leq   g'(\gamma) \leq \left(1 + \kappa_1\right)^{-3} \left(\kappa_1^2 - \frac{(1 + \kappa_1)}{\kappa_1 \left(1 +d\right)}\right).
\end{align*}

Finally, this gives the bound for the overall result
\begin{align}\label{eqn:grad:g}
    | g'(\gamma)| \leq \left(1 + \kappa_1\right)^{-3} \cdot \max\left( \left| 1 - \frac{\kappa_1^3 \cdot (1 + \kappa_1)}{1 + d \kappa_1} \right|, \left| \kappa_1^2 - \frac{(1 + \kappa_1)}{\kappa_1 \left(1 + d\right)} \right| \right).    
\end{align}
Thus, we have
\begin{align*}
  | h'(g(\gamma)) \cdot  g'(\gamma) |  \leq \left(\kappa^2 - \frac{1}{1 + \|R\|}\right)  \cdot 
   \left(1 + \kappa_1\right)^{-3} \cdot \max\left( \left| 1 - \frac{\kappa_1^3 \cdot (1 + \kappa_1)}{1 + d \kappa_1} \right|, \left| \kappa_1^2 - \frac{(1 + \kappa_1)}{\kappa_1 \left(1 + d\right)} \right| \right),    
\end{align*}
where $d\geq 2$ and $\kappa \geq 1$ and $\kappa_1 \geq 1$.

\begin{align}\label{eqn:comps2}
 g(\gamma) = \frac{\sum_{i=1}^n \frac{s_i^2}{(1+\gamma s_i)^2}}{\sum_{i=1}^n \frac{s_i^2}{(1+\gamma s_i)^2}+ (\sum_{i=1}^n s_i)\sum_{i=1}^n \frac{s_i}{(1+\gamma s_i)^2}}. 
\end{align}
Let the scalar functions $h: \mathbb{R}_{+} \to \mathbb{R}_{+}$ and $g: \mathbb{R}_{+} \to \mathbb{R}_{+}$ be defined as
\begin{subequations}
\begin{align}
   %h(g(\gamma))=  \frac{\sum_{i=1}^n \frac{\la_ia_i^2}{(1+  g(\gamma) \la_i)^2}}{\sum_{i=1}^n \frac{a_i^2}{(1+g(\gamma)  \la_i)^2}}, \quad \textnormal{and} \quad
 % g(\gamma)=\frac{\sum_{i=1}^d \frac{s_i^2}{(1+\gamma s_i)^2}}{\sum_{i=1}^d \frac{s_i^2}{(1+\gamma s_i)^2}+ (\sum_{i=1}^d s_i)\sum_{i=1}^d \frac{s_i}{(1+\gamma s_i)^2}},
 h(\bar{\gamma})&= \sum_{i=1}^n \frac{\la_ia_i^2}{ \left(1+ \bar{\gamma} \la_i\right)^2} \left(\sum_{i=1}^n \frac{a_i^2}{\left(1+ \bar{\gamma}  \la_i\right)^2}\right)^{-1},\\
  g(\gamma)&=\left( 1+ \sum_{i=1}^d s_i \left(\sum_{i=1}^d \frac{s_i^2}{\left(1+\gamma s_i\right)^2}\right)^{-1} \sum_{i=1}^d \frac{s_i}{\left(1+\gamma s_i\right)^2}\right)^{-1}.
\end{align}
\end{subequations}

In the following, we verify the two conditions:
\begin{enumerate}[label={\textnormal{\textbf{I\arabic*}}}, wide, labelindent=0pt, itemsep=0pt]
    \item \label{item:i1}
    \item \label{item:i2}  
\end{enumerate}

We note that the gradient \( \frac{\partial h}{\partial g} \) is
\begin{equation}
    \begin{split}
\frac{\partial h}{\partial g} = &-2 \sum_{i=1}^n \frac{\lambda_i^2 a_i^2}{(1 + g \lambda_i)^3} \sum_{i=1}^n \frac{a_i^2}{(1 + g \lambda_i)^2}  \left( \sum_{i=1}^n \frac{a_i^2}{(1 + g \lambda_i)^2} \right)^{-2}\\
&+ 2  \sum_{i=1}^n \frac{\lambda_i a_i^2}{(1 + g \lambda_i)^2} \sum_{i=1}^n \frac{a_i^2 \lambda_i}{(1 + g \lambda_i)^3} \left( \sum_{i=1}^n \frac{a_i^2}{(1 + g \lambda_i)^2} \right)^{-2}. \\
&\yl{= -\sum_{i,j}^n \frac{a_i^2a_j^2(\lambda_i -\lambda_j)^2}{(1 + g \lambda_i)^3(1 + g \lambda_j)^3}  \left( \sum_{i=1}^n \frac{a_i^2}{(1 + g \lambda_i)^2} \right)^{-2}}\\
&\yl{= -\sum_{i,j}^n \frac{a_i^2a_j^2(\lambda_i -\lambda_j)^2}{(1 + g \lambda_i)^3(1 + g \lambda_j)^3}  \left( \sum_{i,j=1}^n \frac{a_i^2a_j^2(1+g\lambda_i)(1+g\lambda_j)}{(1 + g \lambda_i)^3(1+g\lambda_j)^3} \right)^{-1}}\\
    \end{split}
\end{equation}
Since the numerator and denominator of \( h(g) \) contain terms involving \( \frac{1}{(1 + g \lambda_i)^2} \) and \( \frac{1}{(1 + g \lambda_i)^3} \), both decrease slowly as \( g \) increases. Therefore, the derivative \( \frac{\partial h}{\partial g} \) is negative and $-1 < \frac{\partial h}{\partial g} < 0$.  Further, the gradient \( \frac{\partial g}{d\gamma} \) can be written as 
\begin{align*}
\frac{\partial g}{\partial \gamma} = -\frac{1}{A(\gamma)^2} \cdot \frac{ \partial A(\gamma)}{d\gamma}, 
\end{align*}
where
\begin{align*}
A(\gamma) = 1+ \tr{\bSi} \left(\sum_{i=1}^d \frac{s_i^2}{\left(\tr{\bSi}+\gamma s_i\right)^2}\right)^{-1} \sum_{i=1}^d \frac{s_i}{\left(\tr{\bSi}+\gamma s_i\right)^2}.
\end{align*}
The individual terms in the sums decrease slowly because the powers of \( (\text{tr}(\Sigma) + \gamma s_i) \) grow in the denominator. Thus, \( g(\gamma) \) decreases slowly with respect to \( \gamma \), making \( \frac{\partial g}{\partial \gamma} \) negative but also small in magnitude $-1 < \frac{\partial g}{\partial \gamma} < 0$. Hence,  
\begin{align}
   \frac{\partial}{\partial } 
\end{align}

It can be seen that that, for a PSD matrix $\bSi$, the function $ g(\gamma)$ defined in \eqref{func:g(gamma)} is strictly  decreasing in $\gamma$. Further, for a PSD matrix $\bSi$, the function 
\begin{equation*}
     h(\bar{\gamma})= \sum_{i=1}^n \frac{\la_ia_i^2}{ \left(1+ \bar{\gamma} \la_i\right)^2} \left(\sum_{i=1}^n \frac{a_i^2}{\left(1+ \bar{\gamma}  \la_i\right)^2}\right)^{-1}+1,
\end{equation*}
is also strictly decreasing in $\bar{\gamma}$. Thus, the function $h(g(\gamma)) - \gamma$ is strictly  decreasing  verifying Condition \ref{item:i1}. On the other hand, we have 
$\lim_{\gamma_1 \rightarrow 0}(h(g(\gamma_1)) - \gamma_1)  > 0 $ and    $ \lim_{\gamma_2 \rightarrow \infty} (h(g(\gamma_2)) - \gamma_2)   <0 $, this verifies Condition \ref{item:i2}.  By the Intermediate Value Theorem, this guarantees the existence of a unique root, denoted as $\gamma = \gamma^\star$.

Hence, using \eqref{eqn:p:opt1} and   \eqref{eqn:w:opt2} we have
\begin{subequations}
\begin{align}
\Pb^\star&:= C (\rb, \bom, \bSi) \cdot \left( \frac{\gamma^\star}{\tr{\bSi}}\cdot \bSi+\Iden \right)^{-1},  \\
\bom^*&:= c (\rb, \bom, \bSi) \cdot\left(  g(\gamma^\star) \cdot \Rb+\Iden\right)^{-1}\rb.
\end{align}    
\end{subequations}
which implies that $\Pb^\star$ and $\bom^*$ are  unique up to multiplicaiton by constants $ C (\rb, \bom, \bSi)$ and $ c(\rb, \bom, \bSi)$.

\begin{lemma}
For the function  $h: \mathbb{R}_{+} \to \mathbb{R}_{+}$ defined as
\begin{equation}
      h(g)= \sum_{i=1}^n \frac{\la_ia_i^2}{ \left(1+g\la_i\right)^2} \left(\sum_{i=1}^n \frac{a_i^2}{\left(1+ g  \la_i\right)^2}\right)^{-1},
\end{equation}
we have  $-1 < \partial h/\partial g \leq 0$. 
\end{lemma}
\begin{proof}
%We first show that $-1 < \frac{\partial h}{\partial g} \leq 0$. 
% \begin{equation}
% \frac{\partial h}{\partial g} = \frac{-2 \left(\sum_{i=1}^n \frac{a_i^2}{(1+g\lambda_i)^2} \sum_{i=1}^n \frac{\lambda_i^2a_i^2}{(1+g\lambda_i)^3} - \sum_{i=1}^n \frac{\lambda_ia_i^2}{(1+g\lambda_i)^2} \sum_{i=1}^n \frac{\lambda_ia_i^2}{(1+g\lambda_i)^3}\right)}{\left(\sum_{i=1}^n \frac{a_i^2}{(1+g\lambda_i)^2}\right)^2}
% \end{equation}
Let
\begin{align*}
A &:= \sum_{i=1}^n \frac{a_i^2}{(1+g\lambda_i)^2}, \qquad B := \sum_{i=1}^n \frac{\lambda_i^2a_i^2}{(1+g\lambda_i)^3}, \\
C &:= \sum_{i=1}^n \frac{\lambda_ia_i^2}{(1+g\lambda_i)^2}, \qquad D := \sum_{i=1}^n \frac{\lambda_ia_i^2}{(1+g\lambda_i)^3}.
\end{align*}
The gradient $\frac{\partial h}{\partial g}$ can be written as 
\begin{align}\label{eqn:grad:g}
 \frac{\partial h}{\partial g}= \frac{-2(AB - CD)}{A^2}.    
\end{align}
We first show that $\frac{\partial h}{\partial g} \leq 0$. To do so, we need to show that $AB \geq CD$. This directly follows from ..
% \begin{equation}\label{eqn:ableqcd}
% AB =\left(\sum_{i=1}^n \frac{a_i^2}{(1+g\lambda_i)^2}\right)\left(\sum_{i=1}^n \frac{\lambda_i^2a_i^2}{(1+g\lambda_i)^3}\right) \geq \left(\sum_{i=1}^n \frac{\lambda_ia_i^2}{(1+g\lambda_i)^{5/2}}\right)^2 = CD.
% \end{equation}
We now show that  $\frac{\partial h}{\partial g} > -1$, which is equivalent to showing  that $-2(AB - CD) > -A^2$. This is equivalent to showing that $2(AB - CD) < A^2$. Using \eqref{eqn:ableqcd}, we get $2(AB - CD) \leq 0 < A^2$ which together with \eqref{eqn:grad:g} implies that $\partial h/ \partial g > -1$.

Finally, we provide the limiting behaviours. As $g \to \infty$, all terms approach 0, so $\frac{\partial h}{\partial g} \to 0$. Further,
   \begin{equation*}
   \lim_{g \to 0} \frac{\partial h}{\partial g} = \frac{-2(\sum a_i^2 \sum \lambda_i^2a_i^2 - (\sum \lambda_ia_i^2)^2)}{(\sum a_i^2)^2}.
   \end{equation*}
This limit is always between -1 and 0 due to the Cauchy-Schwarz inequality. We have shown that $-1 < \frac{\partial h}{\partial g} \leq 0$ for all non-negative $a_i$, $\lambda_i$, and $g$.
\end{proof}

\begin{lemma}
There exist $\gamma_1, \gamma_2 \in \mathbb{R}_{+}$ such that $(h(g(\gamma_1)) - \gamma_1) \cdot (h(g(\gamma_2)) - \gamma_2) < 0$. 
\end{lemma}

\end{proof}
