# Supplementary material for: Gating is Weighting: Understanding Gated Linear Attention through In-context Learning
Source: arXiv:2504.04308 source file (2025-04-06)
Supplement: Supplementary file 6 [file supp_unique.tex]

% \subsection{Proof of Uniqueness}

% Recap the loss and gradient from \eqref{app:loss}, \eqref{app:gd P} and \eqref{app:gd w}. Let $M:=\tr{\bSi}+\sigma^2$. 
% For simplification and without loss of generality, let $\Pt=\sqrt{\bSi}\Pb\sqrt{\bSi}$. Then we obtain
% \begin{align*}
%     \Lc(\Pt,\bom)=M-2\tr{\bSi\Pt}\bom^\top\rb+M\tn{\bom}^2\tr{\Pt^\top\Pt}+(\tn{\bom}^2+\bom^\top\Rb\bom)\tr{\bSi\Pt^\top\Pt}.\\
% \end{align*}
% and
% \begin{align*}
% &\nabla_{\Pt}\Lc(\Pt,\bom)=-2\bom^\top\rb\bSi+2M\tn{\bom}^2\Pt+2(\tn{\bom}^2+\bom^\top\Rb\bom)\bSi\Pt\\
% &\nabla_{\bom}\Lc(\Pt,\bom)=-2\tr{\bSi\Pt}\rb+2M\tr{\Pt^\top\Pt}\bom+2\tr{\bSi\Pt^\top\Pt}(\Iden_n+\Rb)\bom.
% \end{align*}
% Then setting $\nabla_{\Pt}\Lc(\Pt,\bom)=0$ and $\nabla_{\bom}\Lc(\Pt,\bom)=0$ returns
% \begin{equation}
%     \begin{split}
%       \Pt&=\left(M\tn{\bom}^2\Iden+(\tn{\bom}^2+\bom^\top\Rb\bom)\bSi\right)^{-1}\bSi\bom^\top\rb\\
%     &=\frac{\bom^\top\rb}{M\tn{\bom}^2}\left(\frac{\tn{\bom}^2+\bom^\top\Rb\bom}{M\tn{\bom}^2}\Iden+\bSi^{-1}\right)^{-1}\\
%     &=\frac{\bom^\top\rb}{M\tn{\bom}^2}\left(\frac{\gamma}{M}\cdot\Iden+\bSi^{-1}\right)^{-1} .     
%     \end{split}
% \end{equation}
% where we set $$\gamma=\frac{\bom^\top\Rb\bom}{\tn{\bom}^2}+1$$ and
% \begin{equation}
% \begin{split}
% \bom&=\left(\left(M\tr{\Pt^\top\Pt}+\tr{\bSi\Pt^\top\Pt}\right)\Iden+\tr{\bSi\Pt^\top\Pt}\Rb\right)^{-1}\tr{\bSi\Pt}\rb\\
%     &=\frac{\tr{\bSi\Pt}}{M\tr{\Pt^\top\Pt}+\tr{\bSi\Pt^\top\Pt}}\left(\Iden+\frac{\tr{\bSi\Pt^\top\Pt}}{M\tr{\Pt^\top\Pt}+\tr{\bSi\Pt^\top\Pt}}\Rb\right)^{-1}.    
% \end{split}
% \end{equation}
% Let 
% \begin{align*}
%  \bSi_{\gamma} := \frac{\gamma}{M}\cdot\Iden + \bSi^{-1}.  
% \end{align*}
% Then we get
% \begin{align*}
%     g(\gamma)&:=\frac{\tr{\bSi\Pt^\top\Pt}}{M\tr{\Pt^\top\Pt}+\tr{\bSi\Pt^\top\Pt}}\\
%     &=\left(1+M\frac{\tr{\Pt^\top\Pt}}{\tr{\bSi\Pt^\top\Pt}}\right)^{-1}\\
%     &=\left(1+M\frac{\tr{\bSi_{\gamma}^{-2}}}{\tr{\bSi\bSi_{\gamma}^{-2}}}\right)^{-1}\\
%     &=\left(1+M\sum_{i=1}^d\frac{s_i^2}{(1+\gamma s_i)^2}\left(\sum_{i=1}^d\frac{s_i^3}{(1+\gamma s_i)^2}\right)^{-1}\right)^{-1}.
% \end{align*}
% Here, the equality follows from  eigen decomposition $\bSi=\Ub \textnormal{diag}(\mathbf{s})\Ub^\top$ with  $\s = [s_1, \ldots, s_d]^\top \in \R^d_{+}$.

% Now, plugging $\Pb$ defined in \eqref{eqn:p:opt1} within $\bom$ given in \eqref{eqn:w:opt1}, we obtain
% \begin{align}\label{eqn:w:opt2}
% \bom = \frac{  \tn{\bom}^2 \tr{\bSi} \tr{\bSi \bSi^{-1}_{\gamma}}}{  \bom^\top\rb  \left( \tr{\bSi  \bSi^{-2}_{\gamma}} + \tr{\bSi} \tr{\bSi  \bSi^{-2}_{\gamma}} \right)} \cdot\left(g(\gamma) \cdot \Rb+\Iden\right)^{-1}\rb.
% \end{align}
% Using the above formulae for $\bom$, we rewrite $\gamma$ in \eqref{eqn:gamma} as
% \begin{equation}\label{eqn:comps1}
% \begin{split}
%     \gamma &= \frac{\rb^\top (  g(\gamma) \Rb+\Iden)^{-1}\Rb(  g(\gamma) \Rb+\Iden)^{-1}\rb}{ \rb^\top (  g(\gamma) \Rb+\Iden)^{-2}\rb} +1\\
% %&= \frac{\sum_{i=1}^n \frac{\la_ia_i^2}{(1+  g(\gamma) \la_i)^2}}{\sum_{i=1}^n \frac{a_i^2}{(1+g(\gamma)  \la_i)^2}}\\
% %&=\left( 1+ \sum_{i=1}^d s_i \left(\sum_{i=1}^d \frac{s_i^2}{\left(1+\gamma s_i\right)^2}\right)^{-1} \sum_{i=1}^d \frac{s_i}{\left(1+\gamma s_i\right)^2}\right)^{-1}\\
% &= \sum_{i=1}^n \frac{\la_ia_i^2}{ \left(1+  g(\gamma) \la_i\right)^2} \left(\sum_{i=1}^n \frac{a_i^2}{\left(1+g(\gamma)  \la_i\right)^2}\right)^{-1}+1\\
% &=: h\left(g\left(\gamma\right)\right),  
% \end{split}    
% \end{equation}
% where the second equality follows since $\Rb = \Eb \text{diag}(\bla) \Eb^\top$ denotes the eigen decomposition of $\Rb$, where $\s = [s_1, \ldots, s_d]^\top \in \R^d_{+}$ and $\bla = [\lambda_1, \ldots, \lambda_n]^\top \in \R^n_{+}$, and by our assumption $\rb = \Eb \ab$ for some $\ab = [a_1, \ldots, a_n]^\top \in \R^n_{+}$.


% \begin{lemma}
% Let the functions \( h: \mathbb{R}_{+} \to \mathbb{R}_{+} \) and \( g: \mathbb{R}_{+}  \to  \mathbb{R}_{+} \) be defined as
% \begin{align}
%       h(\bar{\gamma}) &= \sum_{i=1}^n \frac{\lambda_i a_i^2}{ \left(1+\bar{\gamma} \lambda_i\right)^2} \left(\sum_{i=1}^n \frac{a_i^2}{\left(1+ \bar{\gamma}  \lambda_i\right)^2}\right)^{-1}, \\
%       g(\gamma) &=  \left(1 + M
% \left( \sum_{i=1}^d \frac{s_i^3}{\left( M+ (\gamma+1) s_i \right)^2} \right)^{-1}
% \sum_{i=1}^d \frac{s_i^2}{\left( M+ (\gamma+1) s_i \right)^2}\right)^{-1}.
% \end{align}
% We have that \( | h'(g(\gamma)) \cdot  g'(\gamma) | < 1 \).
% \end{lemma}
% \begin{proof}
% % Let the scalar function $g: \mathbb{R}_{+} \rightarrow \mathbb{R}_{+}$ be defined by
% % \begin{equation}\label{func:g(gamma)}
% %     \begin{split}
% %  g(\gamma) &:= \left( 1+ M \left(\sum_{i=1}^d \frac{s_i^3}{\left(M+\gamma s_i\right)^2}\right)^{-1} \sum_{i=1}^d \frac{s_i^2}{\left(M+\gamma s_i\right)^2}\right)^{-1} \\
% % %  &=  \left( 1+ M \left(\sum_{i=1}^d \frac{s_i^3}{D_i(\gamma)^2}\right)^{-1} \sum_{i=1}^d \frac{s_i^2}{D_i(\gamma)^2}\right)^{-1}.
% %     \end{split}
% % \end{equation}
% Let  \( D_i(\gamma) = M + (\gamma+1) s_i \).
% We have
% \[
% B(\gamma) = \sum_{i=1}^d \frac{s_i^3}{D_i(\gamma)^2}, \quad C(\gamma) = \sum_{i=1}^d \frac{s_i^2}{D_i(\gamma)^2}, \quad A(\gamma) = 1 + M \frac{C(\gamma)}{B(\gamma)}.
% \]
% The derivatives of \( B(\gamma) \) and \( C(\gamma) \) are
% \[
% B'(\gamma) = -2 \sum_{i=1}^d \frac{s_i^4}{D_i(\gamma)^3}, \quad C'(\gamma) = -2 \sum_{i=1}^d \frac{s_i^3}{D_i(\gamma)^3}.
% \]
% The gradient of \( g(\gamma) \) is
% \begin{equation}\label{eqn:partialg}
% \begin{split}
%  g'(\gamma) &= - \frac{M }{A(\gamma)^2} \cdot \frac{C'(\gamma) B(\gamma) - C(\gamma) B'(\gamma)}{B(\gamma)^2}.
% % & =- \frac{M }{A(\gamma)^2 B(\gamma)^2} \cdot \left(C'(\gamma) B(\gamma) - C(\gamma) B'(\gamma)\right).        
% \end{split}
% \end{equation}
% It can be seen that 
% \begin{equation*}
%     \begin{split}
%  \frac{1}{A^2(\gamma)}&\leq M^{-2}\left(\sum_{i=1}^d \frac{s_i^3}{D_i(\gamma)^2} \right)^2 \cdot \left(\sum_{i=1}^d \frac{s_i^2}{ D_i(\gamma)^2}\right)^{-2},\\
%     \frac{1}{B^2(\gamma)}&\leq  \left(\sum_{i=1}^d \frac{s_i^3}{D_i(\gamma)^2}\right)^{-2},       
%     \end{split}
% \end{equation*}
% which implies that 
% \begin{subequations}
% \begin{equation}\label{eqn:partial:parta}
%      \frac{1 }{A(\gamma)^2 B(\gamma)^2} \leq M^{-2}  \left(\sum_{i=1}^d \frac{s_i^2}{ D_i(\gamma)^2}\right)^{-2}= M^{-2}  \left(\sum_{i=1}^d \frac{s_i^2 D_i(\gamma)}{ D_i(\gamma)^3}\right)^{-2}.    
% \end{equation}
% Further, we have
% \begin{equation}\label{eqn:partial:partb}
% M\left(C'(\gamma) B(\gamma) - C(\gamma) B'(\gamma)\right)= M^2 \sum_{i=1}^d \sum_{j=1}^d \frac{s_i^2 s_j^2 (s_i-s_j)^2}{D_i(\gamma)^3 D_j(\gamma)^3}.    
% \end{equation}
% \end{subequations}
% Note that $D_i(\gamma) \cdot D_j(\gamma) \geq (s_i-s_j)^2$ for all $i, j \in [d]$. Hence, substituting \eqref{eqn:partial:parta}--\eqref{eqn:partial:partb} into   \eqref{eqn:partialg} gives $\abs{\partial g/\partial \gamma} <1$. 

% Let
% \begin{align*}
% A(g) &:= \sum_{i=1}^n \frac{\lambda_i a_i^2}{(1+g\lambda_i)^2}, \qquad A'(g) := -2 \sum_{i=1}^n \frac{\lambda_i^2 a_i^2}{(1+g\lambda_i)^3}, \\
% B(g) &:= \sum_{i=1}^n \frac{a_i^2}{(1+g\lambda_i)^2}, \qquad B'(g) := -2 \sum_{i=1}^n \frac{\lambda_i a_i^2}{(1+g\lambda_i)^3}.
% \end{align*}
% The derivative of $h$ with respect to \( g \) is given by
% \begin{align*}
%      \frac{\partial h}{\partial g} = \frac{B(g)A'(g) - A(g)B'(g)}{B(g)^2}.
% \end{align*}
% We begin by bounding each term in \( \frac{\partial h}{\partial g} \). First, observe that


% We note that the gradient \( \frac{\partial h}{\partial g} \) is
% \begin{equation}
%     \begin{split}
% \frac{\partial h}{\partial g} = &-2 \sum_{i=1}^n \frac{\lambda_i^2 a_i^2}{(1 + g \lambda_i)^3} \sum_{i=1}^n \frac{a_i^2}{(1 + g \lambda_i)^2}  \left( \sum_{i=1}^n \frac{a_i^2}{(1 + g \lambda_i)^2} \right)^{-2}\\
% &+ 2  \sum_{i=1}^n \frac{\lambda_i a_i^2}{(1 + g \lambda_i)^2} \sum_{i=1}^n \frac{a_i^2 \lambda_i}{(1 + g \lambda_i)^3} \left( \sum_{i=1}^n \frac{a_i^2}{(1 + g \lambda_i)^2} \right)^{-2}. \\
% &= -\sum_{i,j}^n \frac{a_i^2a_j^2(\lambda_i -\lambda_j)^2}{(1 + g \lambda_i)^3(1 + g \lambda_j)^3}  \left( \sum_{i=1}^n \frac{a_i^2}{(1 + g \lambda_i)^2} \right)^{-2}\\
% &= -\sum_{i,j}^n \frac{a_i^2a_j^2(\lambda_i -\lambda_j)^2}{(1 + g \lambda_i)^3(1 + g \lambda_j)^3}  \left( \sum_{i,j=1}^n \frac{a_i^2a_j^2(1+g\lambda_i)(1+g\lambda_j)}{(1 + g \lambda_i)^3(1+g\lambda_j)^3} \right)^{-1}, 
%     \end{split}
% \end{equation}
% which implies that \( |\frac{\partial h}{\partial g}| <1 \). 
% \end{proof}
